# Supplementary material for: The role of orbital angular momentum constraints in the variational optimization of the two-electron reduced-density matrix
Source: arXiv:1906.00922 ancillary file (2019-06-03)
Supplement: Supplementary file 1 [file si.pdf]

# Supporting information for: The role of orbital angular momentum constraints in the variational optimization of the two-electron reduced-density matrix

Run R. Li[1] and A. Eugene DePrince III[1]

[1] *Department of Chemistry and Biochemistry, Florida State University, Tallahassee, FL 32306-4390*

## I. SECOND-ROW ATOMS

Table SI reports absolute energies of second-row atoms determined by the direct variational optimization of the two-electron reduced-density matrix (2-RDM) and the full configuration interaction (CI) method. All variational 2-RDM (v2RDM) computations were performed under two-particle $N$-representability conditions. Numerical values listed under the heading "Real" were obtained from v2RDM computations using real-valued reduced-density matrices (RDMs). Numerical values listed under the headings $\mathrm{L}^2$ and $\mathrm{L_z}$ were obtained from complex-valued v2RDM computations enforcing constraints on the expectation value of $\hat{L}^2$ or the expectation values of $\hat{L}^2$ and $\hat{L}_z$, respectively. The percent error in the correlation energy is defined as $(E_{\mathrm{v2RDM}} - E_{\mathrm{CI}})/(E_{\mathrm{CI}} - E_{\mathrm{Hartree-Fock}}) \times 100\%$. The missing data correspond to excited states for which Hartree–Fock or real-valued v2RDM solutions cannot be obtained. All computations were performed within the cc-pVDZ basis set. The convergence thresholds employed within the v2RDM computations are outlined in the main text. These standard thresholds could not be met in all cases; cases for which more loose criteria were employed are indicated by superscripts in Table SI.

TABLE I: Absolute v2RDM-derived energies ($E_\mathrm{h}$) for second row atoms and the corresponding percent errors in the correlation energy. All errors are relative to values obtained from full CI computations.

| | | Energy/$E_\mathrm{h}$ (Percent error of correlation energy) | | | | | | |
|---|---|---|---|---|---|---|---|---|
| Atom | Term | Real | | $L^2$ | | $L_z$ | | full CI |
| Li | $^2$S | -7.4326 | (0.2) | -7.4326 | (-0.7) | -7.4326 | (-3.7) | -7.4326 |
| Be | $^1$S | -14.6175 | (0.2) | -14.6175 | (0.1) | -14.6175 | (0.1) | -14.6174 |
| Be | $^3$P | -14.5164 | (1.8) | -14.5164 | (1.5) | -14.5164 | (0.7) | -14.5164 |
| B | $^2$P | -24.5933 | (4.1) | -24.5929 | (3.6) | -24.5913 | (1.0) | -24.5906 |
| B | $^4$P | -24.4626 | (7.8) | -24.4621 | (4.0) | -24.4618 | (1.2) | -24.4616 |
| C | $^3$P | -37.7690 | (8.9) | -37.7685 | (8.3) | -37.7641 | (2.8) | -37.7619 |
| C | $^1$D | -37.7373 | (26.9) | -37.7251 | (16.0) | -37.7111 | (3.4) | -37.7073 |
| C | $^1$S | – | – | -37.6656 | – | -37.6656 | – | -37.6542 |
| C | $^5$S | -37.6179 | (1.2) | -37.6179 | (1.3) | -37.6178 | (1.2) | -37.6175 |
| N | $^4$S | -54.4836 | (3.8) | -54.4836 | (3.8) | -54.4836 | (3.8) | -54.4801 |
| N | $^2$D | -54.4194 | (29.8) | -54.4076 | (20.8) | -54.3890 | (6.7) | -54.3802 |
| N | $^2$P | – | – | -54.3764 | – | -54.3585[a] | – | -54.3364 |
| N | $^4$P | – | – | -54.2828 | – | -54.0705 | – | -54.0672 |
| O | $^3$P | -74.9449 | (26.7) | -74.9431 | (25.2) | -74.9261 | (11.6) | -74.9117 |
| O | $^1$D | -74.8872 | (32.3) | -74.8802 | (28.1) | -74.8515 | (11.0) | -74.8330 |
| O | $^1$S | – | – | -74.7858 | – | -74.7858 | – | -74.7538 |
| F | $^2$P | -99.5715 | (26.6) | -99.5706 | (26.1) | -99.5546[a] | (15.9) | -99.5295 |
| F | $^4$P | -98.2868 | (25.1) | -98.2854 | (24.5) | -98.2684[a] | (16.9) | -98.2302 |
| Ne | $^1$S | -128.7085 | (14.4) | -128.7086 | (14.4) | -128.7086 | (14.4) | -128.6809 |

[a] Loose convergence criterial were employed ($\epsilon_\mathrm{gap} < 5.6 \times 10^{-4}\mathrm{E_h}$ and $\epsilon_\mathrm{error} < 4.4 \times 10^{-6}$).

## II. MOLECULAR OXYGEN

Table SII reports the energies for multiple spin and angular momentum states of molecular oxygen, computed at the full CI, multireference CI (MRCISD+Q), and v2RDM levels of theory. All values are given relative to the energy of the $^3\Sigma$ state, as described by the relevant level of theory. Values listed under the headings $\mathrm{L}_z$ and $(\Delta \mathrm{L}_z)^2$ were obtained from v2RDM computations in which constraints were placed on the expectation value of $\hat{L}_z$ or the expectation value and variance of $\hat{L}_z$, respectively. The convergence thresholds employed within the v2RDM computations are outlined in the main text. These standard thresholds could not be met in all cases; cases for which more loose criteria were employed are indicated by superscripts in Table SII.

TABLE II: The relative energies (eV) of the spin and orbital angular momentum states of molecular oxygen described by the STO-3G, D95V, and cc-pVDZ basis sets. All energies are given relative to that of the $^3\Sigma$ state.

| | STO-3G | | | d95v | | | cc-pVDZ | | |
|---|---|---|---|---|---|---|---|---|---|
| | full CI | $L_z$ | $(\Delta L_z)^2$ | MRCISD+Q | $L_z$ | $(\Delta L_z)^2$ | MRCISD+Q | $L_z$ | $(\Delta L_z)^2$ |
| $^1\Sigma$ | 1.60 | 0.91 | 1.39 | 1.66 | 0.38 | 0.88 | 1.71 | -0.19 | 0.52 |
| $^1\Pi$ | 9.68 | 0.92 | 8.51[a] | 9.08 | 0.47 | 2.13[b] | 9.45 | -0.04 | 1.52[e] |
| $^1\Delta$ | 1.04 | 1.03 | 1.04 | 1.14 | 1.16 | 1.19 | 1.05 | 0.93 | 0.95 |
| $^3\Sigma$ | 0 | 0 | 0 | 0 | 0 | 0 | 0 | 0 | 0 |
| $^3\Pi$ | 8.30 | 3.01 | 8.27 | 7.69 | 2.90 | 6.24[c] | 8.05 | 2.70 | 5.70[f] |
| $^3\Delta$ | 6.20 | 6.30 | 6.30 | 6.30 | 6.55 | 6.57 | 6.30 | 6.47 | 6.48 |
| $^5\Sigma$ | 16.89 | 15.67 | 16.95 | 14.64 | 13.68 | 14.64[d] | 15.37 | 14.11 | 15.09[g] |
| $^5\Pi$ | 15.59 | 15.70 | 15.70 | 13.87 | 14.06 | 14.07 | 14.37 | 14.65 | 14.65 |
| $^5\Delta$ | 22.49 | 22.60 | 22.60 | 20.62 | 20.91 | 20.93 | 21.38 | 21.78 | 21.78 |

[a] Loose convergence criteria were employed ($\epsilon_{\rm gap} < 6.5 \times 10^{-4}$ $E_h$, $\epsilon_{\rm error} < 1.4 \times 10^{-6}$).

[b] Loose convergence criteria were employed ($\epsilon_{\rm gap} < 3.8 \times 10^{-4}$ $E_h$, $\epsilon_{\rm error} < 3.2 \times 10^{-6}$).

[c] Loose convergence criteria were employed ($\epsilon_{\rm gap} < 8.3 \times 10^{-4}$ $E_h$, $\epsilon_{\rm error} < 1.2 \times 10^{-5}$).

[d] Loose convergence criteria were employed ($\epsilon_{\rm gap} < 1.3 \times 10^{-4}$ $E_h$, $\epsilon_{\rm error} < 4.1 \times 10^{-6}$).

[e] Loose convergence criteria were employed ($\epsilon_{\rm gap} < 9.3 \times 10^{-4}$ $E_h$, $\epsilon_{\rm error} < 5.4 \times 10^{-6}$).

[f] Loose convergence criteria were employed ($\epsilon_{\rm gap} < 2.0 \times 10^{-3}$ $E_h$, $\epsilon_{\rm error} < 1.4 \times 10^{-5}$).

[g] Loose convergence criteria were employed ($\epsilon_{\rm gap} < 2.8 \times 10^{-4}$ $E_h$, $\epsilon_{\rm error} < 3.6 \times 10^{-6}$).
